# Supplementary material for: Hierarchical Inducing Point Gaussian Process for Inter-domain Observations
Source: arXiv:2103.00393 source file (2021-06-24)
Supplement: Supplementary file 1 [file uk-time-comparison.tex]

\begin{tabular}{lrrrrrrrrrr}
    \toprule
    %{} & \multicolumn{5}{c}{M} \\
    M &   1{,}600 & 3{,}600 & 6{,}400 & 10{,}000 & 14{,}400 & 19{,}600 &  25{,}600 & 32{,}400 & 40{,}000 \\
    \midrule
    HIP-GP (RMSE)& 0.438 &   0.423 &   0.420 &   0.411 & 0.409 & 0.400 &0.397 &0.393 & 0.389 \\
    SVGP (RMSE) & 0.437 &   0.423 &   0.420 &   0.412 & 0.409 & 0.398 &0.396 & n/a & n/a \\
   % KISS-GP (RMSE) & 0.433 & 0.418 & 0.408 & 0.400& 0.400& 0.393 & 0.391 & 0.389 &  0.387 \\
    \midrule
    HIP-GP (time) & 27.7         &41.52          &65.7          &\textbf{91.2}  &\textbf{115.7} &\textbf{119.8} &\textbf{130.7} &\textbf{129.5} &\textbf{133.2} \\
    SVGP (time)   &\textbf{12.0} &\textbf{22.5} &\textbf{45.6} &193.6          &406.3 &668.1 &898.2 &n/a &n/a\\
    \bottomrule %\\
    \end{tabular}
